# Supplementary material for: Tunable spin and transport in porphyrin-graphene nanoribbon hybrids
Source: arXiv:2210.13610 source file (2022-10-24)
Supplement: Supplementary file 1 [file Supplementary-Material.pdf]

# Supplementary Material:

# Tunable spin and transport in porphyrin-graphene nanoribbon hybrids

Fei Gao[1], Rodrigo E. Menchón [2], Aran Garcia-Lekue [2,3] and Mads Brandbyge[1]

[1] Department of Physics, Technical University of Denmark, DK-2800 Kongens Lyngby, Denmark
[2] Donostia International Physics Center (DIPC), 20018 Donostia-San Sebastián, Spain
[3] IKERBASQUE, Basque Foundation for Science, 48013 Bilbao, Spain

## Figures

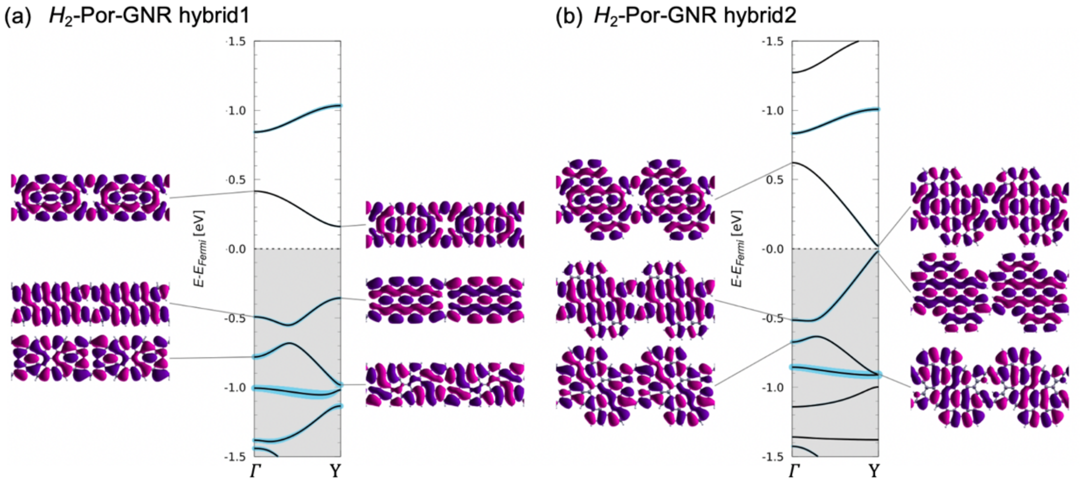


Figure S1 Electronic band structures of (a) $H_2$-Por-GNR hybrid1 and (b) $H_2$-Por-GNR hybrid2, together with the wavefunctions at Γ and Y of the most relevant states around Fermi level. Light and dark magenta clouds indicate the positive and negative sign of the wave-functions, respectively. Isosurfaces with values of 0.02 e/bohr$^3$are shown.

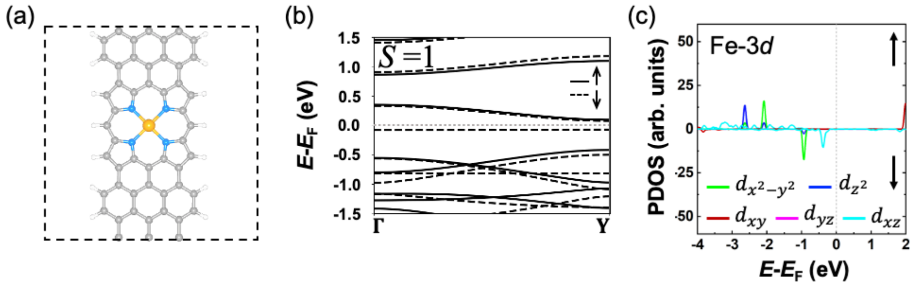


Figure S2 (a) The optimized structures of Fe-Por-GNR hybrid1, (b) its band structure and (c) DOS projected on Fe atom.

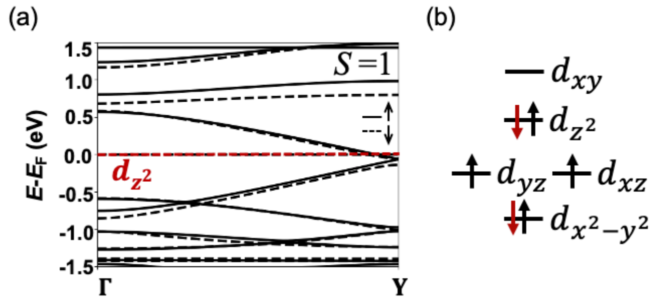


Figure S3 Another possible electronic configuration of Fe atom in Fe-Por-GNR hybrid2, $(d_{x^2-y^2})^2(d_{z^2})^2(d_{xz})^1(d_{yz})^1$: (a) Band structure and (b) Occupation of Fe $d$-orbitals. Here, the $d_{z^2}$ orbital is just at the Fermi level.

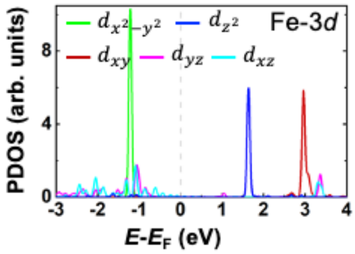


Figure S4 DOS projected on Fe atom upon attachment of a CO molecule. The whole system now is non-magnetic.
